# Supplementary material for: No-Regret Learning in Bayesian Games
Source: arXiv:1507.00418 source file (2015-11-19)
Supplement: Supplementary file 1 [file appendix_bce.tex]

\begin{defn}[Bayes-Correlated Equilibrium - $\BCE$]\label{defn:bce}
A randomized strategy profile $\sr\in \Delta(\Sigma)$ is a Bayes-correlated Equilibrium if for every $s_i'\in \Sigma_i\rightarrow \Sigma_i$:
\begin{equation}
\E_{\sr}\E_{\vr}\left[U_i(\sr(\vr); \vr_i)\right] \geq \E_{\sr}\E_{\vr}\left[U_i(s_i'(\vr_i,\sr_i),\sr_{-i}(\vr_{-i}); \vr_i)\right]
\end{equation}
\end{defn}

Last, we also describe the concept of an \emph{Agent-Form Bayes-Correlated Equilibrium} ($\ABCE$) (c.f. Forges \cite{Forges1993}), which is similar to $\BCE$, with the restriction that the deviation conditional on a value $v_i$, can only depend on the previous action $s_i(v_i)$ and not on the whole strategy $s_i$. In the definition of a $\BCE$, we assume that the player does not regret switching to some other strategy $s_i'$ whenever he was using strategy $s_i$. Thus the switch $s_i'$ can be viewed as a function of the whole strategy $s_i$, in other words, the deviating action $a_i'=s_i'(v_i)$ of a player with value $v_i$ can depend on the action that a player with value $v_i'$ was previously playing. The $\ABCE$ does not allow for such dependence. Hence, the set of $\ABCE$ is a superset of $\BCE$. 

\begin{figure}\label{fig:incomplete-comparison}
\centering
\input{incomplete-comparison.pstex_t}
\caption{Comparison among static solution concepts in the incomplete information setting and connection to no-regret learning under incomplete information.}
\end{figure}

\begin{defn}[Agent-Form Bayes-Correlated Equilibrium - $\ABCE$]\label{defn:abce}
A randomized strategy profile $\sr\in \Delta(\Sigma)$ is a Bayes-correlated Equilibrium if for any $i\in [n]$, $v_i\in \V_i$ and $a_i':\A_i\rightarrow \A_i$:
\begin{equation}
\E_{\sr}\E_{\vr| \vr_i=v_i}\left[U_i(\sr(\vr); \vr_i)\right] \geq \E_{\sr}\E_{\vr| \vr_i=v_i}\left[U_i(a_i'(\sr_i(\vr_i)),\sr_{-i}(\vr_{-i}); \vr_i)\right]
\end{equation}
\end{defn}

Observe that a $\BCCE$ is a superset of $\ABCE$, since the type of deviations allowed in the definition of a $\BCCE$ belong to the class of deviations allowed in the definition of a 
$\ABCE$. Thus the stability restrictions are weaker under a $\BCCE$. Figure \ref{fig:incomplete-comparison} depicts the comparison of the different solution concepts related to games of incomplete information.
